# Supplementary material for: Time-Sensitive Importance Splitting
Source: arXiv:2506.19568 source file (2025-06-24)
Supplement: Supplementary file 1 [file 95-appendix.tex]

\appendix

\section{IOSA Models of Repariable Fault Trees}

\gd{Should we include them?}

\cb{nahhh, they can check it in the artifact\ldots\ unless it helps explain why exploration depths $\in[10,18]$ are the most efficient in our experiments, then yes we can add them here}
